# Supplementary material for: Spontaneous rotation and propulsion of suspended capsules in active nematics
Source: arXiv:2510.17643 source file (2025-10-20)
Supplement: Supplementary file 1 [file SM.pdf]

# Supplementary Material: Spontaneous rotation and propulsion of suspended capsules in active nematics

Júlio P. A. Santos,[1,2,3] Margarida M. Telo da Gama,[1,2,4] and Rodrigo C. V. Coelho[1,2,5,*]

[1]*Centro de Física Teórica e Computacional, Faculdade de Ciências, Universidade de Lisboa, 1749-016 Lisboa, Portugal.*

[2]*Departamento de Física, Faculdade de Ciências, Universidade de Lisboa, P-1749-016 Lisboa, Portugal.*

[3]*University of Vienna, Faculty of Physics, Kolingasse 14-16, 1090 Vienna, Austria*

[4]*International Institute for Sustainability with Knotted Chiral Meta Matter, Hiroshima University, Higashihiroshima 739-8511, Japan.*

[5]*Centro Brasileiro de Pesquisas Físicas, Rua Xavier Sigaud 150, 22290-180 Rio de Janeiro, Brazil*

(Dated: October 15, 2025)

## ACTIVE NEMATICS MODEL

## METHODS

### Hydrodynamic equations

We describe active nematics within a two-dimensional continuum hydrodynamic framework, summarized here. The local orientational state is represented by the director field $\mathbf{n}(\mathbf{x})$, which specifies the mean particle alignment at position $\mathbf{x}$. The degree of order is quantified by the scalar order parameter $S$, with $S = 0$ in the isotropic phase and a finite value $S_N$ in the nematic phase. Because particles are apolar, the appropriate order parameter is the symmetric, traceless tensor

$$Q_{\alpha\beta} = 2S\left(n_\alpha n_\beta - \delta_{\alpha\beta}/2\right). \tag{1}$$

In the free-energy description, bulk ordering contributions are omitted. Such a choice is motivated by experiments on microtubule–kinesin suspensions, where nematic order arises solely from activity. Similar modeling assumptions have been used in earlier works [1–3]. The free-energy density includes (i) an elastic contribution penalizing distortions in the order parameter, $f_E = K(\partial_\gamma Q_{\alpha\beta})^2/2$, with $K$ the elastic constant, and (ii) an anchoring term at solid boundaries, $f_W = W(Q_{\alpha\beta} - Q^0_{\alpha\beta})^2/2$, which enforces the surface-preferred order $Q^0_{\alpha\beta}$ with anchoring strength $W$. The total free energy is then

$$\mathcal{F} = \int f\, d^2x, \tag{2}$$

where $f = f_E + f_W$ at surfaces and $f = f_E$ elsewhere.

The dynamics couples nematic order to flow through the Beris–Edwards equation for $Q_{\alpha\beta}$, the incompressibility condition, and the Navier–Stokes equation for the velocity field $\mathbf{v}$ [4–6]:

$$\partial_t Q_{\alpha\beta} + v_\gamma \partial_\gamma Q_{\alpha\beta} - S_{\alpha\beta} = \Gamma H_{\alpha\beta}, \tag{3}$$

$$\partial_\alpha v_\alpha = 0, \tag{4}$$

$$\rho\partial_t v_\alpha + \rho v_\beta \partial_\beta v_\alpha = -\partial_\alpha p + 2\eta\partial_\beta D_{\alpha\beta} - \zeta\partial_\beta Q_{\alpha\beta} - \chi v_\alpha. \tag{5}$$

Here $\Gamma$ is the rotational diffusivity, $H_{\alpha\beta}$ the molecular field,

$$H_{\alpha\beta} = -\frac{\delta\mathcal{F}}{\delta Q_{\alpha\beta}} + \frac{\delta_{\alpha\beta}}{2}\,\mathrm{Tr}\left(\frac{\delta\mathcal{F}}{\delta Q_{\gamma\epsilon}}\right), \tag{6}$$

and $S_{\alpha\beta}$ the co-rotational contribution,

$$\begin{aligned} S_{\alpha\beta} &= (\xi D_{\alpha\gamma} + W_{\alpha\gamma})(Q_{\beta\gamma} + \delta_{\beta\gamma}/2) \\ &\quad + (Q_{\alpha\gamma} + \delta_{\alpha\gamma}/2)(\xi D_{\gamma\beta} - W_{\gamma\beta}) \\ &\quad - 2\xi\,(Q_{\alpha\beta} + \delta_{\alpha\beta}/2)\,(Q_{\gamma\epsilon}\partial_\gamma v_\epsilon). \end{aligned} \tag{7}$$

The vorticity and rate-of-strain tensors are $W_{\alpha\beta} = (\partial_\beta v_\alpha - \partial_\alpha v_\beta)/2$ and $D_{\alpha\beta} = (\partial_\beta v_\alpha + \partial_\alpha v_\beta)/2$, respectively. The parameter $\xi$ controls flow alignment and depends on particle shape: $\xi > 0$ for rod-like and $\xi < 0$ for disk-like nematogens. In this study, rod-like particles in the flow-aligning regime are considered. In Eq. (5), $\rho$ is the fluid density, $p$ the pressure, $\chi$ is the friction coefficient with the substrate, $\eta$ the shear viscosity, and $\zeta$ the activity coefficient (positive for extensile systems). This model corresponds to a simplified but standard 2d description of active nematics [1, 6, 7]. Since active stresses dominate over passive ones in most relevant conditions [8], passive contributions to the stress tensor are neglected as in previous studies [2, 9].

**Numerical implementation**

The simulations employ a hybrid algorithm: Eq. (3) is integrated with a predictor–corrector finite-difference scheme, while Eqs. (4) and (5) are recovered in the macroscopic limit using the lattice Boltzmann method [7, 10]. Capsules impose no-slip and weak planar anchoring conditions, implemented with the immersed-boundary lattice Boltzmann method [11, 12], a lattice Boltzmann compatible variation of the immersed-boundary method [13]. The filled suspended bodies were also implemented using the same immersed-boundary lattice Boltzmann method, using a triangular mesh to fill the equivalent capsule shapes.

The system is initialized with fluid at rest and directors approximately aligned along the horizontal axis, perturbed by random fluctuations of $\pm 2°$. Random seeds are varied across simulations. Parameter values are expressed in lattice units (l.u.), where the lattice spacing $\Delta x = 1$, the time step $\Delta t = 1$, and the reference density $\rho_0 = 1$. In these units, the chosen parameters are: fluid density $\rho = 40$, viscosity $\eta = 6.67$, elastic constant $K = 0.015$, aligning parameter $\xi = 0.9$, activity $\zeta = 0.04$, anchoring strength $W = 0.002$, rotational diffusivity $\Gamma = 0.4$, and friction coefficient $\chi = 0.02$.

**Fluid-capsule interaction: Immersed Boundary method (IBM)**

The immersed-boundary method takes advantage of the Lagrangian and Eulerian representations of the same system, using the Lagrangian points to resolve the solid points' motion and an Eulerian grid to represent the hydrodynamics. Assuming conservation of mass, incompressibility, and uniform viscosity, one can represent the discretized dynamics of a system of a purely kinetic fluid and a purely elastic material by [13]

$$\rho\left(\frac{\partial \mathbf{u}}{\partial t} + S_h(\mathbf{u})\mathbf{u}\right) + \mathbf{D}^0_{h,b}p = \mu L_h \mathbf{u} + \mathbf{f} \tag{8}$$

$$\mathbf{D}^0_{h,b} \cdot \mathbf{u} = 0 \tag{9}$$

$$\rho(\mathbf{x},t) = \sum_{(q,r,s)\in G_h} M(q,r,s)\delta_h\left(\mathbf{x} - \mathbf{x}(q,r,s,t)\right)\Delta q \Delta r \Delta s \tag{10}$$

$$\mathbf{f}(\mathbf{x},t) = \sum_{(q,r,s)\in G_h} \mathbf{f}(q,r,s,t)\delta_h\left(\mathbf{x} - \mathbf{x}(q,r,s,t)\right)\Delta q \Delta r \Delta s \tag{11}$$

$$\frac{\partial \mathbf{x}}{\partial t}(q,r,s,t) = \sum_{\mathbf{x}\in g_h} \mathbf{u}(\mathbf{x},t)\delta_h\left(\mathbf{x} - \mathbf{x}(q,r,s,t)\right)h^3 \tag{12}$$

$$\mathbf{f}\Delta q \Delta r \Delta s = -\frac{\partial}{\partial \mathbf{x}(q,r,s)} U_h(...\mathbf{x}(q',r',s',t)...). \tag{13}$$

,

where $\rho$, $\mathbf{u}$, and $\mathbf{f}$ are the Eulerian density, velocity, and force, respectively; $M$, $\mathbf{X}$, and $\mathbf{F}$ are the Lagrangian point mass, position, and force, respectively. The Lagrangian force is calculated from the elastic potential energy of the elastic material, and then propagated to the Eulerian space using (10). The Eulerian velocity is calculated from the hydrodynamic equations (8 and 9), and then propagated to the Lagrangian space. Since these hydrodynamic equations are a discretized form of the incompressible Navier-Stokes equation, it has been shown that one can use lattice Boltzmann to solve the hydrodynamics and obtain the Eulerian velocities. With this, one can couple a purely elastic material to a lattice Boltzmann fluid simulation. The discrete delta Dirac, $\delta_h$, present in (10-12) must follow strict rules, to *hide* the discrete grid effects as much as possible [13]. For a compromise between precision and efficiency, we chose the 4-point delta function,

$$\phi(r) = \phi_4(r) = \begin{cases} \frac{1}{8}\left(3 - 2|r| + \sqrt{1 + 4|r| - 4|r|^2}\right) & 0 \leq |r| \leq 1 \\ \frac{1}{8}\left(5 - 2|r| - \sqrt{-7 + 12|r| - 4|r|^2}\right) & 1 \leq |r| \leq 2 \\ 0 & |r| > 2. \end{cases} \quad (14)$$

This function will have an impact on the size and shape of the capsule's membrane, as it will give it a "virtual width", as opposed to being a 1d smooth line. We will use $h = 1$, as the fluid lattice size and consider only two spatial dimensions,

$$\delta_h(\mathbf{x}) = \phi_4(x)\phi_4(y). \quad (15)$$

**Capsules**

Capsules are 1d closed membranes of different shapes and elastic properties with fluid in- and outside. We describe the membranes as a finite number of points - nodes - connected by a straight line to their first neighbors. The interaction between first neighbors follows an elastic potential energy [12, 14],

$$U = U_{stretch} + U_{bending} + U_{area}. \quad (16)$$

This takes into account:

*stretching*,

$$\begin{aligned} U_{\text{stretch}} &= \frac{1}{2}k_s \sum_j (l_j - l_{j0})^2, \\ l_j &= x_{j+1} - x_j \ \text{ for } j < n_n, \\ l_{n_n} &= x_0 - x_{n_n}, \end{aligned} \quad (17)$$

maintaining the preferred distance between nodes, and taking into account non-linear behavior observed in biological capsules/cells [15];

*bending*,

$$U_{bending} = k_b \sum_j \left[1 - \cos\left(\theta_j - \theta_{j0}\right)\right], \quad (18)$$

maintaining the angle defined by three consecutive nodes;

and *conservation of volume*,

$$U_{\text{area}} = \frac{1}{2}k_a \frac{(A - A_0)^2}{A_0}, \quad (19)$$

maintaining the 2d volume of the capsule.

The force felt by a node $i$ is given by,

$$\mathbf{f}_i = \boldsymbol{\nabla}_i U. \tag{20}$$

It is generally best to keep the distance between the nodes as one lattice unit $\Delta x$ [16], and so we distribute $\lceil n_{\rm nodes} \rceil$ equidistant points along the desired capsule shape. We choose the node closest to $(D/2, 0)$ to represent the symmetry axis, from the center of mass to that node. Figures S1 - S3 show the capsule shapes and the chosen symmetry axis.

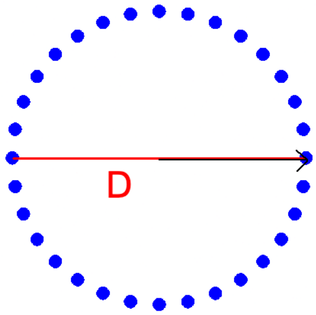


FIG. S1: Example of a circular capsule, and the corresponding capsule's axis of symmetry (black arrow) - although arbitrary, this was chosen to be consistent with the axes of symmetry of the other shapes. The red line corresponds to the size (diameter) of the capsule, $D$.

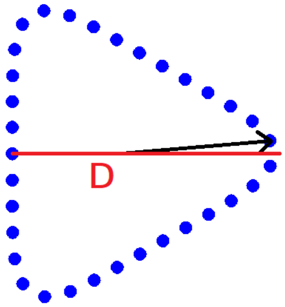


FIG. S2: Example of a triangular capsule, and the corresponding symmetry axis (black arrow) - although arbitrary, this was chosen to be consistent with the axes of symmetry of the other shapes. The red line corresponds to the size of the capsule, $D$.

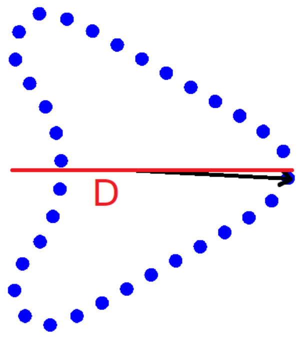


FIG. S3: Boomerang-shaped capsule constructed from an initially triangular shape, and corresponding symmetry axis (black arrow). The red line corresponds to the size of the capsule, $D$.

**Numerical implementation of IB-LBM for a capsule immersed in an active nematic fluid**

We take $h = \Delta q = \Delta r = \Delta s = 1$. The index $i$ is used to refer to a capsule node, e.g. the position of node $i$ is represented as $\mathbf{x}_i$. Time steps are represented by the $n$ upper index, which is given by $n = \frac{t}{\Delta t}$, e.g. the position of node $i$ at time $t = n\Delta t$ is represented as $\mathbf{x}_i^n$.

The whole iteration will be:

1. Set the anchoring directions around the capsule (applied in step 6). Each lattice point's anchoring angle is defined as a weighted average of the angles of its nearest capsule faces (the lines connecting consecutive nodes). Weights are assigned so that closer faces greater influence the anchoring direction. Angles are first measured relative to the $x$-axis, and after averaging, converted into unit vectors that define the local anchoring directions.

2. Set the velocity of the capsule's points as, (12),

$$\frac{\partial \mathbf{x}^n}{\partial t}_i = \sum_{\mathbf{x}\in g_h} \mathbf{v}^n(\mathbf{x})\delta_h\left(\mathbf{x} - \mathbf{x}_i^n\right); \tag{21}$$

3. Move the capsule's points half a step using a simple Euler method, $n \to n + \frac{1}{2}$,

$$\mathbf{x}_i^{n+\frac{1}{2}} = \mathbf{x}_i^n + \frac{\Delta t}{2}\frac{\partial \mathbf{x}^n}{\partial t}_i; \tag{22}$$

4. Calculate the force felt by the capsule points, arising from the potentials in (16),

$$\mathbf{f}_i^{n+\frac{1}{2}} = -\nabla_i U; \tag{23}$$

5. Spread the force to the fluid,

$$\mathbf{f}_{\text{capsule}}^{n+\frac{1}{2}}(\mathbf{x}) = \sum_i \mathbf{f}_i^{n+\frac{1}{2}} \delta_h(\mathbf{x} - \mathbf{x}_i^{n+\frac{1}{2}}); \tag{24}$$

6. Solve the Beris-Edwards equation (3), with planar anchoring at the capsule, using the order parameter of the previous time step $\mathbf{Q}^{n-1}(\mathbf{x})$ and the anchoring preferential directions saved from step 1, to obtain the values of $\mathbf{Q^n}(\mathbf{x})$;

7. Compute the force due to the active stresses $\Pi = \zeta \mathbf{Q}^n(\mathbf{x})$ and the nematic friction force $\mathbf{f}_\chi{}^n(\mathbf{x}) = -\chi \mathbf{v}^n(\mathbf{x})$,

$$\mathbf{f}_{\text{nematic}}^n(\mathbf{x}) = -\zeta \boldsymbol{x} \cdot \mathbf{Q}^n(\mathbf{x}) - \chi \mathbf{v}^n(\mathbf{x}); \tag{25}$$

8. Compute the LBM collisions, taking into account the force $\mathbf{f}^n(\mathbf{x}) = \mathbf{f}_{\text{capsule}}^{n+\frac{1}{2}} + \mathbf{f}_{nematic}^{n+\frac{1}{2}}$;

9. Iterate the LBM distribution functions in time;

10. Set the new velocity of the capsule's points at the half step as,

$$\frac{\partial \mathbf{x}^{n+\frac{1}{2}}}{\partial t}_i = \sum_{\mathbf{x} \in g_h} \mathbf{v}^{n+1}(\mathbf{x}) \delta_h \left( \mathbf{x} - \mathbf{x}_i^{n+\frac{1}{2}} \right), \tag{26}$$

where $\mathbf{v}^{n+1}(\mathbf{x})$ is the average fluid velocity during the iteration;

11. Finally, move the capsule points a whole step,

$$\mathbf{x}_i^{n+1} = \mathbf{x}_i^n + \Delta t \frac{\partial \mathbf{x}^{n+\frac{1}{2}}}{\partial t}_i; \tag{27}$$

12. Repeat from 1.

**Simulation parameters**

All simulations were iterated $2 \times 10^5$ times before introducing the capsule into the system. After this initial step, to reach the fluid steady state, we set the time to $t = 0$ and iterated $10^6$ time steps. The sample averages considered 120 samples with different random initial conditions.

- The lattice-Boltzmann parameters used were: box size $L_x = L_y = 1024$ with periodic boundary conditions (PBC), characteristic time $\tau = 1$ – which corresponds to viscosity $\eta = 6.67$ with the BGK collision scheme –, and density $\rho = 40$.
- The values of the active nematic, used to solve the Beris-Edwards equation, were: elastic constant $K = 0.015$, aligning parameter $\xi = 0.9$, activity $\zeta = 0.04$, anchoring strength $W = 0.002$, rotational diffusivity $\Gamma = 0.4$, and friction coefficient $\chi = 0.02$.
- The coefficients used for the elastic potentials of the capsules were: stretching $k_s = 1.7k$, bending $k_b = 1.1k$, and area conservation $k_A = 5.55 \times 10^{-4}$. The parameter $k$ was used to adjust flexibility, where $k = 100$ was taken as the rigid limit.

Unless otherwise specified, all reported quantities are given in these units. A connection with physical dimensions can be established by comparing dimensionless ratios or characteristic scales from simulations with their experimental counterparts. As an example, length scales in active nematics are naturally set by the average defect separation $D_{def}$ [17], which can be measured directly both in experiments and in simulations. Under typical experimental conditions, an unconfined active nematic exhibits a characteristic spacing of $D_{def} \approx 70\,\mu$m [18]. In simulations with the present parameter set, the corresponding distance is $D_{def} \approx 25\,\Delta x$. This comparison yields the mapping $1\,\Delta x \approx 2.8\,\mu$m, which can be used to convert lengths. In the same simulations of active nematics, the average velocity of the system is $v_r = 0.0101$ and the density is $\rho_r = 40$. Those three quantities together can be measured both in simulations and experiments and used to convert all other mechanical quantities.

## CALCULATION OF THE ACTIVE FORCE ON THE REAR OF A BOOMERANG CAPSULE

The propulsion of boomerang-shaped capsules can be understood from the active stress contribution,

$$\sigma^{\mathrm{a}}_{ij} = -\zeta\, Q_{ij}, \tag{28}$$

with activity coefficient $\zeta$ and nematic tensor $Q_{ij}$. The corresponding force density is

$$f_i = \partial_j \sigma^{\mathrm{a}}_{ij} = -\zeta\, \partial_j Q_{ij}. \tag{29}$$

For a constant scalar order parameter $S$, $Q_{ij}$ may be written as

$$Q_{ij} = S\,(2n_i n_j - \delta_{ij}), \tag{30}$$

with $\mathbf{n}$ the director field. Under planar anchoring at the capsule boundary, $\mathbf{n}$ coincides with the local tangent vector $\mathbf{t}$. Spatial variations of $\mathbf{t}$ occur along the arc length $s$, and the Frenet–Serret relation gives $\partial_s \mathbf{t} = \kappa \nu$, where $\kappa = 1/R$ is the local curvature and $\nu$ here denotes the outward surface normal. Substituting, one finds

$$\partial_j Q_{ij} = 2S\,\kappa\,\nu_i, \tag{31}$$

and therefore

$$f_i = -2\zeta S\,\kappa\,\nu_i. \tag{32}$$

Equation (32) shows that the local active force density points along the surface normal and scales linearly with curvature. Integrating this density over a circular arc of radius $R$ and opening angle $\Delta\theta$ yields the net propulsion force along the capsule symmetry axis:

$$F \;\simeq\; 4\,\zeta S\,\sin\!\left(\tfrac{\Delta\theta}{2}\right), \tag{33}$$

per unit depth in the out-of-plane direction (2d). For small openings ($\Delta\theta \ll 1$), this reduces to $F \approx 2\zeta S\,\Delta\theta$. In the special case of a semicircular rear ($\Delta\theta = \pi$), the result is particularly simple: $F = 4\zeta S$.

## AVERAGE DISTANCE BETWEEN DEFECTS

The topological charge density can be calculated from the nematic field, as

$$q(\mathbf{r}) \;=\; \frac{1}{2\pi}\Big(\partial_x Q_{xx}\,\partial_y Q_{xy} - \partial_x Q_{xy}\,\partial_y Q_{xx}\Big). \tag{34}$$

This relation was used to calculate the charge density over the whole lattice, which was then divided into two regimes: positively-charged lattice points, where $q(\mathbf{r}) > 0$; and negatively-charged lattice points, where $q(\mathbf{r}) < 0$. Then, the number, $N_+$ ($N_-$), of positive (negative) defects was estimated by dividing the value of the total positive (negative) charge by $1/2$ ($-1/2$) – the charge of a single defect. From this, one can estimate the average distance between defects, $d$, using

$$d \;=\; \sqrt{\frac{L_x L_y}{N_+ + N_-}}. \tag{35}$$

## AVERAGE VELOCITY OF THE ACTIVE FLUID

The average velocity of the active fluid, $v_r$, was calculated using the values for the velocity field taken every $5 \times 10^4$ iterations, in a total of 21 measurements,

$$v_r = \frac{1}{N_T} \sum_t \left(\frac{1}{L_x L_y} \sum_i ||\mathbf{v}_i||\right)(t), \tag{36}$$

where $\mathbf{v}_i$ refers to the velocity at the lattice point $i$, $N_T$ to the number of measurements, and $(\frac{1}{L_x L_y} \sum_i ||\mathbf{v}_i||)(t)$ to the average velocity of the system at time $t$.

Since we only introduce the capsule in the box after the initial buffer of $2 \times 10^4$ iterations, and the corresponding average velocity at $t = 0$ is equal to the velocity at any other measured time, we can conclude that the capsule does not interfere with the global dynamics of the active nematic, most likely due to the small size of the capsule, when compared to the size of the system (Fig. S5). The size of the simulation box was $1024 \times 1024$ with periodic boundary conditions, and the buffer of $2 \times 10^4$ was shown to be sufficient to reach the steady state. These measurements were made with a circular capsule of size $D = 25$, but we found the same values for other shapes and sizes.

## TIME-AVERAGED 2d HISTOGRAMS

The time-averaged 2d histograms were obtained by selecting a square region centered on the capsule's center of mass. For each frame, the region was translated and rotated so that its center coincided with the origin and the capsule's symmetry axis was aligned with the $x$-axis,

$$\mathbf{X}_i^{\text{stabilized}}(t) = \mathbf{R}(-\theta(t))\mathbf{T}(-\mathbf{X}_{\text{center}}(t))\mathbf{X}_i(t), \tag{37}$$

$$\mathbf{R}(\theta(t)) = \begin{bmatrix} \cos\theta(t) & -\sin\theta(t) & 0 \\ \sin\theta(t) & \cos\theta(t) & 0 \\ 0 & 0 & 1 \end{bmatrix}, \quad \mathbf{T}(\mathbf{X}_{\text{center}}(t)) = \begin{bmatrix} 1 & 0 & x_{\text{center}}(t) \\ 0 & 1 & y_{\text{center}}(t) \\ 0 & 0 & 1 \end{bmatrix}, \tag{38}$$

$$\theta(t) = \text{arctan2}\left[\mathbf{e}_d(t), \quad \mathbf{X}_i(t)\right] = \begin{bmatrix} x_i(t) \\ y_i(t) \\ 1 \end{bmatrix}, \tag{39}$$

$$\tag{40}$$

where $\mathbf{R}$ is a rotation matrix and $\mathbf{T}$ a translation matrix in the $xy$-plane. The rotation aligns the capsule symmetry axis, $\mathbf{e}_d$, with the $x$-axis: we calculate the angle, at time $t$, $\theta(t)$ between $\mathbf{e}_d(t)$ and $\mathbf{e}_x = (1,0,0)$, and perform a rotation of $-\theta(t)$. The coordinates, at time $t$, of the lattice point $X_i(t)$ and the center of the square region $X_{\text{center}}(t)$ are projected into 3d space, so that we can represent the translation operator as a matrix. For the velocity field, we also rotate the vectors accordingly,

$$\mathbf{V}_i^{\text{stabilized}}(t) = \mathbf{R}(-\theta)\mathbf{V}_i(t), \tag{41}$$

$$\mathbf{V}_i(t) = \begin{bmatrix} v_{x,i}(t) \\ v_{y,i}(t) \\ 1 \end{bmatrix}, \tag{42}$$

$$\tag{43}$$

here the projection of the velocity to 3d space was made for consistency with the previous equations.

Once the regions were centered and rotated, for every 500 iterations, (see Fig. S4), we interpolated and summed all values onto a square grid of the original size with twice the resolution. Dividing this by the number of summed steps we get the time-averaged values for the charge density and velocity field at each point in the square grid. The interpolation was made by choosing the grid points closest to each of the lattice points.

## DEFINITIONS: MSD, SA-TAMSD, MSAD, AND $(\text{MSD})_d$

Let us define sample average,

$$\langle(\cdot)\rangle = \frac{1}{N_S}\sum_{1}^{N_S}(\cdot), \tag{44}$$

where $N_S$ is the number of samples, in our case, the number of simulations with different seeds with the same initial conditions and $(\cdot)$ is a generic quantity.

We define the mean squared displacement (MSD), the sample-averaged time-averaged mean squared displacement (SA-TAMSD), the mean squared angle displacement (MSAD), and the mean squared displacement in the direction of the symmetry axis of the capsule,

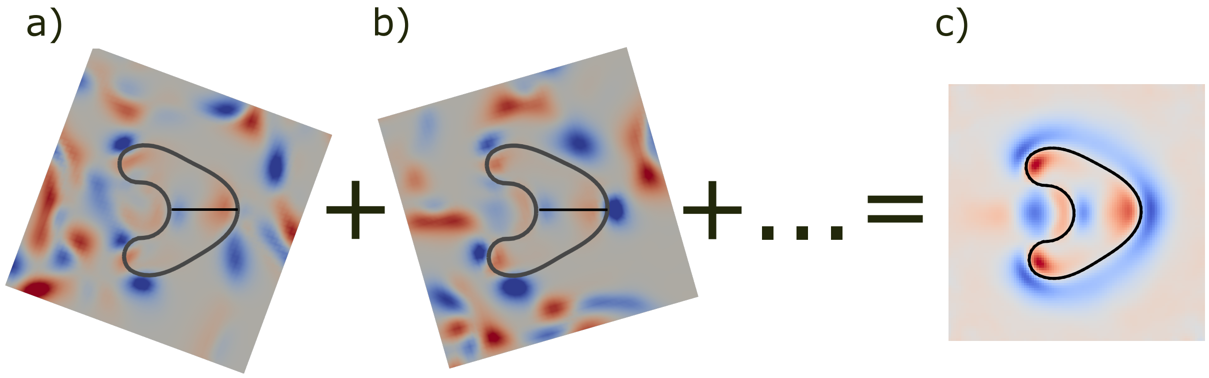


FIG. S4: Visualization of the construction of a 2d time-averaged topological charge density histogram for a boomerang-shaped capsule. In a) and b) there are two examples of centered and rotated images for a boomerang capsule at two distinct time steps of the same simulation, where the black line is the axis of symmetry. After the interpolation of the values to a square grid, and division by the number of summed time steps, we obtain c) the 2d time-averaged topological charge density histogram. Red corresponds to positive, gray to neutral, and blue to negative topological charge density.

$(\mathrm{MSD})_d$, as

$$\begin{aligned}
\mathrm{MSD}(t) &= \left\langle (\mathbf{x}(t) - \mathbf{x}_0)^2 \right\rangle, \\
\text{SA-TAMSD}(t) &= \langle \text{ TAMSD } (t) \rangle, \\
\mathrm{TAMSD}(\tau) &= \frac{1}{T-\tau} \int_0^{T-\tau} [\vec{x}(t+\tau) - \vec{x}(t)]^2 dt \\
\mathrm{MSAD}(t) &= \left\langle (\theta(t) - \theta_0)^2 \right\rangle, \\
(\mathrm{MSD})_d(t) &= \left\langle \left[ \int_0^t (\mathbf{v}(s) \cdot \mathbf{e}_d(s)) ds \right]^2 \right\rangle
\end{aligned}$$

, where $\mathbf{x}$ is the position at time $t$ of the center of mass of the capsule and $\mathbf{x}_0 = \mathbf{x}(0)$. For the TAMSD, $T$ is the total time of the simulation and $\tau$ a lag time. The angle $\theta(t)$ is taken as the angle between the capsule's axis of symmetry at time $t$, $\mathbf{e}_d(t)$ (defined in the section Capsules), and the $x$-axis and $\theta_0 = \theta(0)$. For the $(\mathrm{MSD})_d$, we integrate the projection of the velocity into the axis of symmetry, $\mathbf{e}_d$, to obtain the displacement along the trajectory that corresponds to the motion along the direction $\mathbf{e}_d$.

## SUPPLEMENTARY VIDEOS

- **video1.avi**. Displacement and rotation of a circular capsule with diameter $D = 25$. The line inside the capsule indicates the symmetry axis connecting the center to a fixed point in the capsule. The background, shown only around the capsule, represents the topological charge density.
- **video2.mp4**. Rotation of a circular capsule with diameter $D = 25$ following its center of mass. The symmetry axis is represented as a solid line, the colors represent the topological charge density, and the green lines indicate the director field.
- **video3.mp4**. Rotation of a triangular capsule with size $D = 25$ following its center of mass. The symmetry axis is represented as a solid line, the colors represent the topological charge density, and the green lines indicate the director field.
- **video4.avi**. Motion of a boomerang-shaped capsule with size $D = 25$. The line inside the capsule indicates the symmetry axis connecting the center to a fixed point in the capsule. The background, shown only around the capsule, represents the topological charge density.
- **video5.mp4**. Director and charge density fields around a boomerang-shaped capsule following its center of mass and symmetry axis. It is an example of the process indicated in Fig. S4.

## SUPPLEMENTARY FIGURES

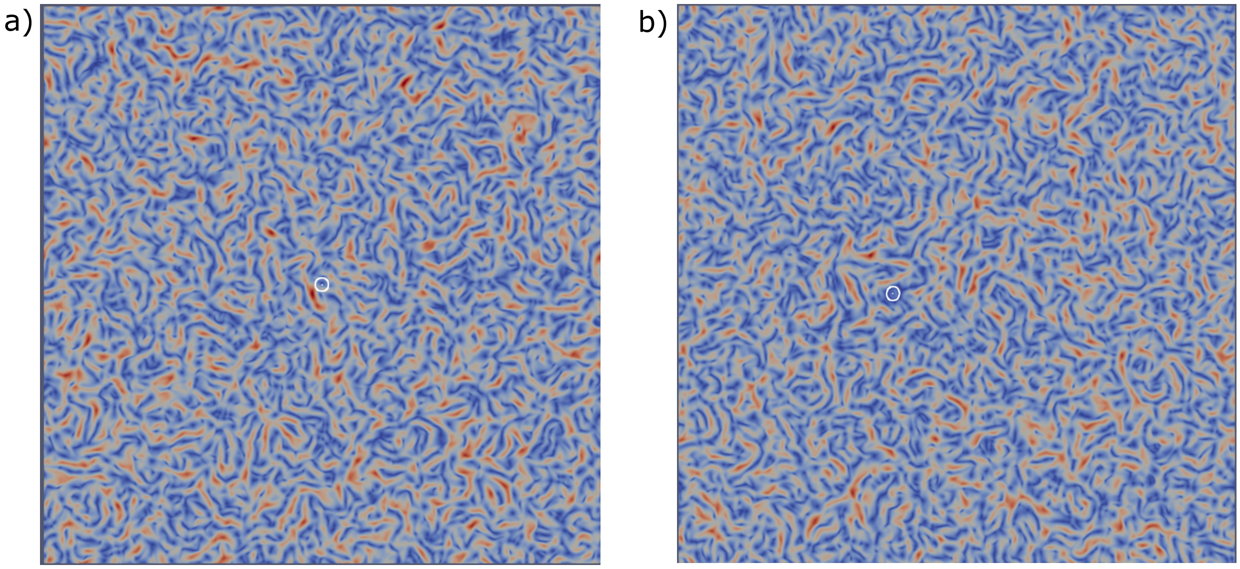


FIG. S5: Example of a typical system, of size $1024 \times 1024$. Velocity field at (a) $2 \times 10^4$ iterations (buffer), when the capsule is released and (b) buffer + $2 \times 10^5$ iterations. The capsule diameter is $D = 25$.

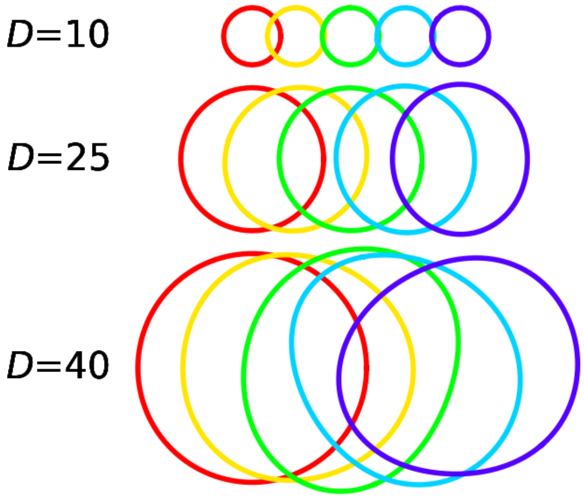


FIG. S6: Example of small deformations for circular capsules with $k = 100$ (rigid limit) of different sizes at $t = 0$ , $2.5 \times 10^5$, $5 \times 10^5$, $7.5 \times 10^5$, $10^6$.

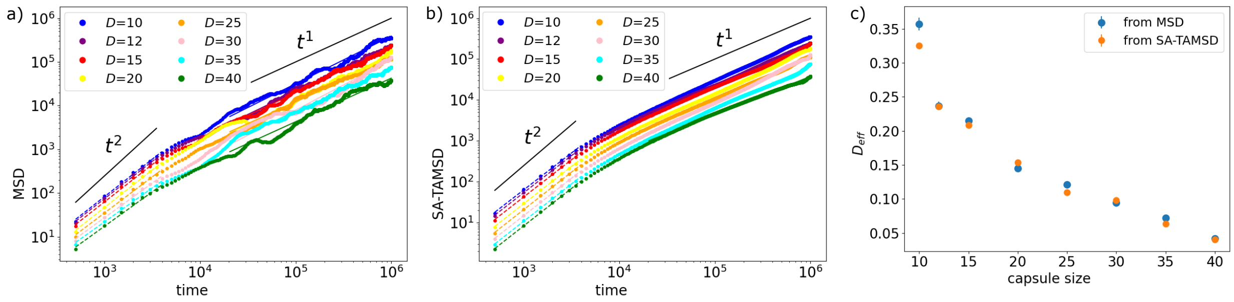


FIG. S7: Displacement of rigid circular capsules of different sizes. (a) Mean squared displacement (MDS). (b) Time-averaged sample-averaged Mean squared displacement (SA-TAMSD). (c) Effective diffusion coefficient as a function of the capsule diameter. See the text for the definitions of MSD and SA-TAMSD.

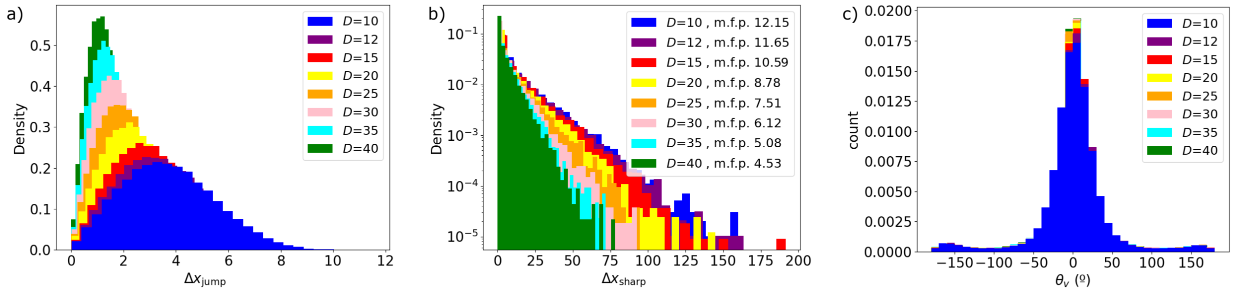


FIG. S8: Distributions for the circular capsules. (a) Probability density function (PDF) for the velocity distribution of capsules of different sizes. $\Delta x_{jump}$, the distance traveled between consecutive intervals of 500 iterations (effective velocity) (b) PDF of the persistence length. Here "m.f.p" means mean free path. $\Delta x_{sharp}$, the distance traveled between sharp turns (persistent length) - change in velocity direction larger than 10° (c) Distribution of angles between consecutive measured velocities.

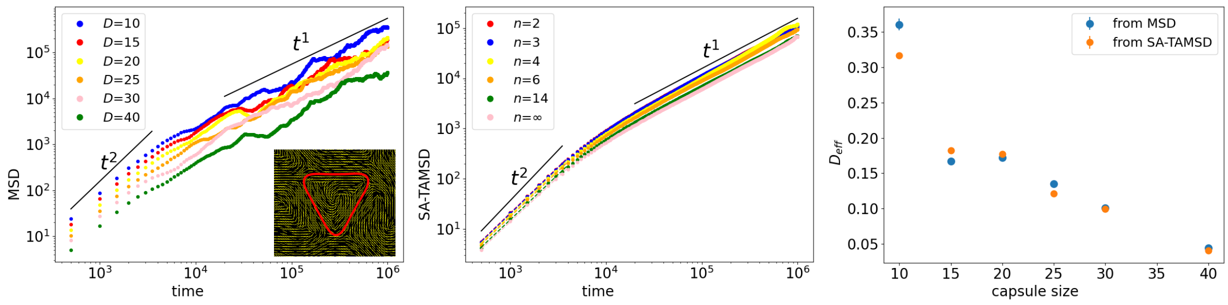


FIG. S9: Displacement of rigid triangular capsules. (a) MSD for capsules of different sizes. The inset depicts a capsule (red) and the director field (yellow lines) at a particular time. (b) SA-TAMSD. (c) Effective diffusion coefficient as a function of size.

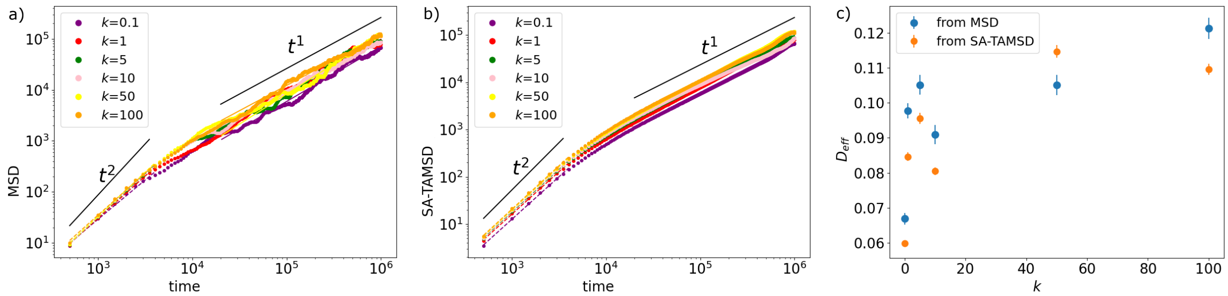


FIG. S10: Displacement of flexible circular capsules with $D = 25$. (a) MSD for different rigidity parameters $k$. (b) Sample-averaged time-averaged MSD. (c) Effective diffusion coefficient as a function of $k$.

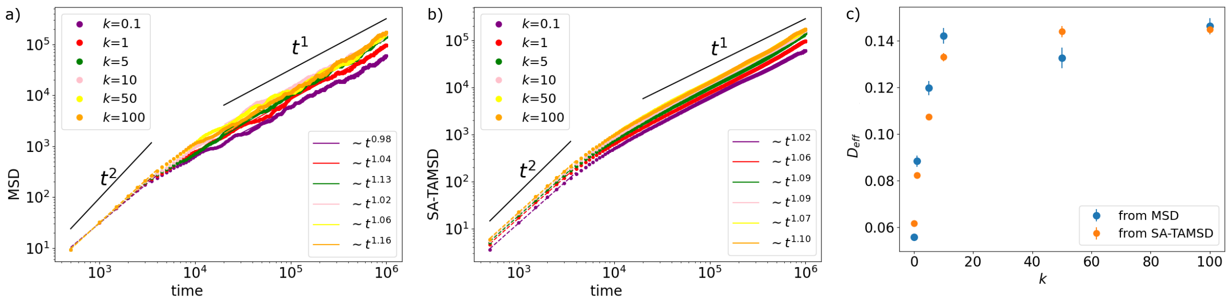


FIG. S11: Displacement of flexible boomerang-shaped capsules of size $D = 25$. (a) MSD for different rigidity parameters $k$. (b) Sample-averaged time-averaged MSD. (c) Effective diffusion coefficient as a function of $k$.

* rcvcoelho@cbpf.br

[1] S. P. Thampi, A. Doostmohammadi, R. Golestanian, and J. M. Yeomans, Europhysics Letters **112**, 28004 (2015).

[2] J. Hardoüin, R. Hughes, A. Doostmohammadi, J. Laurent, T. Lopez-Leon, J. M. Yeomans, J. Ignés-Mullol, and F. Sagués, Communications Physics **2**, 10.1038/s42005-019-0221-x (2019).

[3] R. C. Coelho, J. A. Moreira, D. M. Pedro, and M. M. T. da Gama, Giant **19**, 100309 (2024).

[4] A. N. Beris and B. J. Edwards, *Thermodynamics of flowing systems: with internal microstructure*, 36 (Oxford University Press, USA, 1994).

[5] R. Aditi Simha and S. Ramaswamy, Phys. Rev. Lett. **89**, 058101 (2002).

[6] A. Doostmohammadi, J. Ignés-Mullol, J. M. Yeomans, and F. Sagués, Nature communications **9**, 3246 (2018).

[7] R. C. V. Coelho, N. A. M. Araújo, and M. M. Telo da Gama, Soft Matter **15**, 6819 (2019).

[8] I. Vélez-Cerón, P. Guillamat, F. Sagués, and J. Ignés-Mullol, Proc. Natl. Acad. Sci. U S A **121**, e2312494121 (2024).

[9] R. Saghatchi, M. Yildiz, and A. Doostmohammadi, Phys. Rev. E **106**, 014705 (2022).

[10] D. Marenduzzo, E. Orlandini, M. Cates, and J. Yeomans, Physical Review E **76**, 031921 (2007).

[11] Z.-G. Feng and E. E. Michaelides, Journal of Computational Physics **195**, 602 (2004).

[12] T. Krüger, H. Kusumaatmaja, A. Kuzmin, O. Shardt, S. Gonçalo, and E. Magnus Viggen, *The Lattice Boltzmann Method* (Springer, 2016).

[13] C. Peskin, Acta Numerica **11**, 479 (2002).

[14] D. P. F. Silva, R. C. V. Coelho, I. Pagonabarraga, S. Succi, M. M. Telo da Gama, and N. A. M. Araújo, Soft Matter **20**, 2419 (2024).

[15] M. Nakamura, S. Bessho, and S. Wada, International Journal for Numerical Methods in Biomedical Engineering **30**, 10.1002/cnm.2587 (2014).

[16] T. Krüger, *Computer Simulation Study of Collective Phenomena in Dense Suspensions of Red Blood Cells under Shear* (Springer, 2012).

[17] L. Giomi, Phys. Rev. X **5**, 031003 (2015).

[18] I. Vélez-Ceron, R. C. V. Coelho, P. Guillamat, M. Telo da Gama, F. Sagués, and J. Ignés-

Mullol, Active nematic pumps (2024), arXiv.2407.09960, arXiv:2407.09960 [cond-mat.soft].
